# Supplementary material for: Anisotropic exchange within decoupled tetrahedra in the quantum breathing pyrochlore Ba3Yb2Zn5O11
Source: arXiv:1601.04104 source file (2016-01-16)
Supplement: Supplementary file 1 [file supp.pdf]

# Supplemental Material for "Anisotropic exchange within decoupled tetrahedra in the quantum breathing pyrochlore $Ba_3Yb_2Zn_5O_{11}$"[*]

J. G. Rau,[1,†] L. S. Wu,[2,‡] A. F. May,[3] L. Poudel,[2,4] B. Winn,[2] V. O. Garlea,[2] A. Huq,[5] P. Whitfield,[5] A. E. Taylor,[2] M. D. Lumsden,[2] M. J. P. Gingras,[1,6,7] and A. D. Christianson[2,4]

[1]*Department of Physics and Astronomy, University of Waterloo, Ontario, N2L 3G1, Canada*
[2]*Quantum Condensed Matter Division, Oak Ridge National Laboratory, Oak Ridge, TN-37831, USA*
[3]*Materials Science & Technology Division, Oak Ridge National Laboratory, Oak Ridge, TN-37831, USA*
[4]*Department of Physics & Astronomy, University of Tennessee, Knoxville, TN-37966, USA*
[5]*Chemical & Engineering Materials Division, Oak Ridge National Laboratory, Oak Ridge, TN 37831, USA*
[6]*Perimeter Institute for Theoretical Physics, Waterloo, Ontario, N2L 2Y5, Canada*
[7]*Canadian Institute for Advanced Research, 180 Dundas Street West, Suite 1400, Toronto, ON, M5G 1Z8, Canada*

(Dated: January 16, 2016)

## I. SAMPLE SYNTHESIS

Polycrystalline samples of $Ba_3Yb_2Zn_5O_{11}$ were synthesized by solid-state reaction in $Al_2O_3$ crucibles. The high-purity reactants (dried $Yb_2O_3$, $BaCO_3$, ZnO) were ground together for 5-10 minutes using an agate milling set in a SPEX SamplePrep Mixer/Mill. The mixture was pressed into pellets, which were initially fired at 1150°C for 25-50 h (in air). Subsequent milling, pellet pressing, and annealing at temperatures up to 1170°C were utilized to promote homogeneity and phase purity in the final product. A slight excess (up to 4 at.%) of Ba and Zn-containing reactants was utilized to minimize the chance of forming Yb-containing impurities.

## II. SPECIFIC HEAT AND MAGNETIC SUSCEPTIBILITY

Magnetization measurements were performed upon cooling in an applied field of 0.1 T, and isothermal magnetization measurements were performed at 1.9 K; Quantum Design's Magnetic Property Measurement System was utilized for magnetic measurements. Specific heat measurements were performed in a Quantum Design Physical Property Measurement System.

The specific heat of $Ba_3Yb_2Zn_5O_{11}$ is shown in Fig. S1. The specific heat of a sample from the same batch used for the inelastic neutron scattering measurements is compared with that from Kimura *et al.* [S1]. Both measurements are consistent with a maximum at ~ 2.4 K.

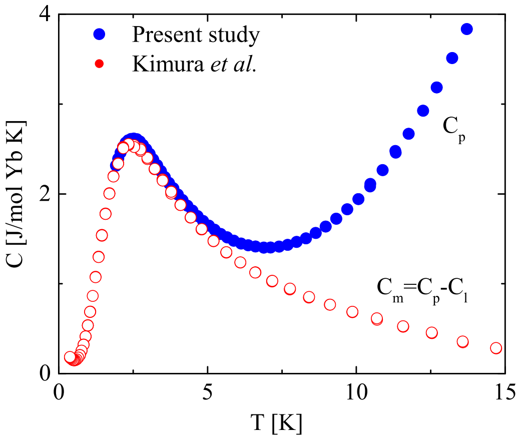


FIG. S1. The temperature dependent specific heat of $Ba_3Yb_2Zn_5O_{11}$. Filled circles are from measurements of a piece taken from the same batch as used for the inelastic neutron scattering measurements. Open circles are the magnetic contribution to the specific heat ($C_m$) taken from Kimura *et al.* [S1], determined $C_m$ by subtracting the lattice contribution ($C_l$) estimated from $Ba_3Lu_2Zn_5O_{11}$ from the specific heat of $Ba_3Yb_2Zn_5O_{11}$ ($C_p$).

The magnetic susceptibility and inverse susceptibility of a sample taken from the same batch as the sample used for the inelastic neutron scattering data are shown in Fig. S2 for an applied field of 0.1 T. A maximum in the susceptibility occurs at ~ 4 K.

## III. NEUTRON DIFFRACTION

Neutron powder diffraction measurements of $Ba_3Yb_2Zn_5O_{11}$ were performed with the time-of-flight powder diffractometer POWGEN, at the Spallation Neutron Source (SNS) at Oak Ridge National Laboratory [S2]. Data were collected on a powder $Ba_3Yb_2Zn_5O_{11}$ sample with mass 6.32 g. The data were collected for 2 hours at temperatures 10 K and 300 K, respectively. Structural refinement was carried out using the software package FULLPROF [S3]

---

* This manuscript has been authored by UT-Battelle, LLC under Contract No. DE-AC05-00OR22725 with the U.S. Department of Energy. The United States Government retains and the publisher, by accepting the article for publication, acknowledges that the United States Government retains a non-exclusive, paid-up, irrevocable, world-wide license to publish or reproduce the published form of this manuscript, or allow others to do so, for United States Government purposes. The Department of Energy will provide public access to these results of federally sponsored research in accordance with the DOE Public Access Plan (http://energy.gov/downloads/doe-public-access-plan).
† jeff.rau@uwaterloo.ca
‡ wul1@ornl.gov

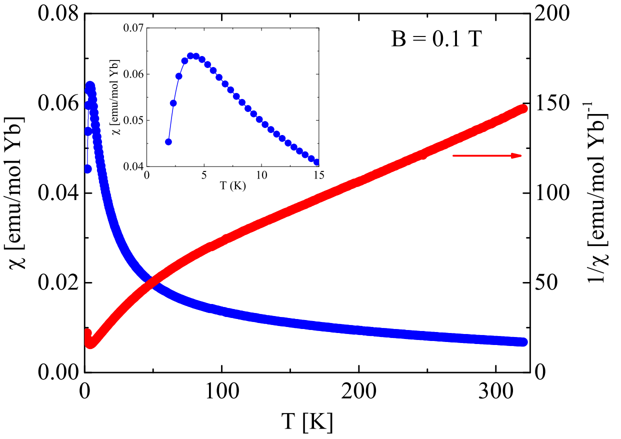


FIG. S2. Left axis: The temperature dependent static magnetic susceptibility ($\chi = M/B$) for $Ba_3Yb_2Zn_5O_{11}$ (blue circles), measured in field $B = 0.1$ T from temperature 1.9 to 320 K. Right axis: The inverse magnetic susceptibility ($1/\chi$) as a function of temperature. The inset shows an expanded view of the low temperature region, where a maximum in the susceptibility occurs around 4 K.

| Atom | Wyckoff | $x$ | $y$ | $z$ | $B_{iso}$ | Occ. |
|---|---|---|---|---|---|---|
| Ba | 24$f$ | 0.7055(3) | 0.00000 | 0.00000 | 0.1313(0) | 0.25000 |
| Yb | 16$e$ | 0.8365(5) | 0.8365(5) | 0.8365(5) | 0.1187(9) | 0.16670 |
| Zn(1) | 16$e$ | 0.0832(5) | 0.0832(5) | 0.0832(5) | 0.1155(4) | 0.16670 |
| Zn(2) | 24$g$ | 0.25000 | 0.25000 | 0.0828(1) | 0.1729(2) | 0.25000 |
| O(1) | 4$b$ | 0.50000 | 0.50000 | 0.50000 | 0.4219(9) | 0.04167 |
| O(2) | 4$a$ | 0.00000 | 0.00000 | 0.00000 | 0.2334(2) | 0.04167 |
| O(3) | 16$e$ | 0.3419(3) | 0.3419(3) | 0.3419(3) | 0.3313(9) | 0.16670 |
| O(4) | 16$e$ | 0.6679(6) | 0.6679(6) | 0.6679(6) | 0.3777(2) | 0.16670 |
| O(5) | 48$h$ | 0.1660(2) | 0.1660(2) | 1.0000(4) | 0.30015(0) | 0.50000 |

| Atom | Wyckoff | $x$ | $y$ | $z$ | $B_{iso}$ | Occ. |
|---|---|---|---|---|---|---|
| Ba | 24$f$ | 0.7055(6) | 0.00000 | 0.00000 | 0.7268(4) | 0.25000 |
| Yb | 16$e$ | 0.8365(5) | 0.8365(5) | 0.8365(5) | 0.4480(3) | 0.16670 |
| Zn(1) | 16$e$ | 0.0832(9) | 0.0832(9) | 0.0832(9) | 0.4184(2) | 0.16670 |
| Zn(2) | 24$g$ | 0.25000 | 0.25000 | 0.0824(7) | 0.5697(8) | 0.25000 |
| O(1) | 4$b$ | 0.50000 | 0.50000 | 0.50000 | 0.8089(3) | 0.04167 |
| O(2) | 4$a$ | 0.00000 | 0.00000 | 0.00000 | 0.4878(2) | 0.04167 |
| O(3) | 16$e$ | 0.3421(4) | 0.3421(4) | 0.3421(4) | 0.6450(5) | 0.16670 |
| O(4) | 16$e$ | 0.6683(0) | 0.6683(0) | 0.6683(0) | 0.7374(4) | 0.16670 |
| O(5) | 48$h$ | 0.1659(4) | 0.1659(4) | 1.0001(6) | 0.6505(3) | 0.50000 |

TABLE S1. Atomic parameters for $Ba_3Yb_2Zn_5O_{11}$ at 10 K (top panel) and 300 K (bottom panel).

The neutron diffraction data at 10 and 300 K along with the Rietveld refinement of the structural model is shown in Fig. S3(a) and (b) respectively. The fitted model describes the data well over a wide wave vector range ($1.3 < |\mathbf{Q}| < 21$ Å$^{-1}$). A few unindexed impurity peaks with intensities less than 1% of the main diffraction peaks of $Ba_3Yb_2Zn_5O_{11}$ are observed. The small fraction of impurities appears to be consistent with that found by Kimura *et al.* [S1] and indicates that the sample consists primarily of the cubic $Ba_3Yb_2Zn_5O_{11}$ phase. No site vacancies or disorder between sites was detected within

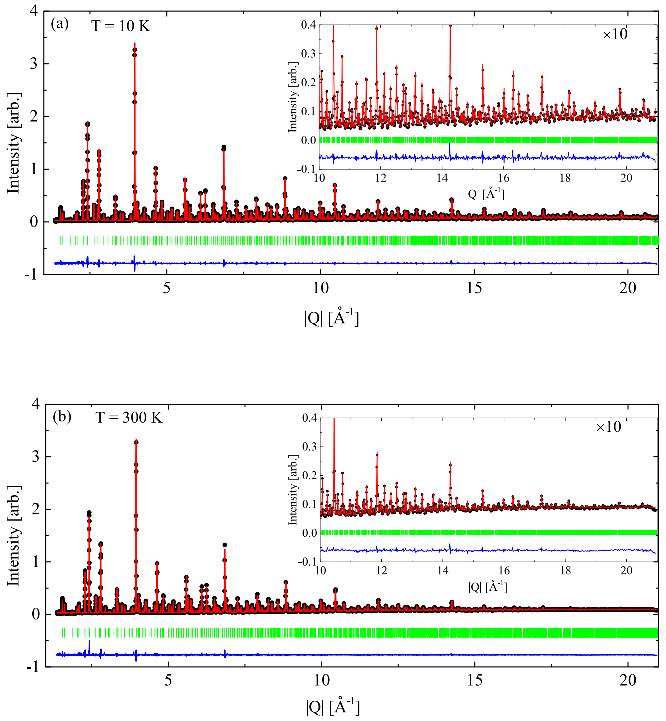


FIG. S3. Neutron powder diffraction data collected with POWGEN at 10 K (a) and 300 K (b) for $Ba_3Yb_2Zn_5O_{11}$. Rietveld refinement (red line), difference pattern (blue line) and calculated reflection positions (green ticks) are superimposed on the data points (black circles). The insets show an expanded view of the high $|\mathbf{Q}|$ region of the data.

| $T$ (K) | $a$ (Å) | $R_p$ | $R_{wp}$ | $R_{exp}$ | $\chi^2$ |
|---|---|---|---|---|---|
| 10 | 13.47117(3) | 9.07 | 8.63 | 1.53 | 31.8 |
| 300 | 13.48997(3) | 10.7 | 9.23 | 1.99 | 21.5 |

TABLE S2. Comparison of the refinement parameters at 10 and 300 K.

experimental resolution. The refined atomic parameters of $Ba_3Yb_2Zn_5O_{11}$ at 10 K and 300 K are shown in Table S1. The lattice constants and goodness of fit parameters are displayed in Table S2.

## IV. INELASTIC NEUTRON SCATTERING

Inelastic neutron scattering (INS) experiments were performed on the hybrid spectrometer (HYSPEC) at the Spallation Neutron Source at Oak Ridge National Laboratory [S5]. The data were collected at 0.25 K, 10 K, and 20 K utilizing a $^3$He refrigerator, with incident energies $E_i$ = 3.8, 7.5, and 15 meV and Fermi chopper frequencies of 180, 300, and 300 Hz respectively. To cover a large region of reciprocal space the center of the detector vessel, which covers 60° of scattering angle, was placed at scattering angles ranging from 33 - 101°.

Shown in Fig. S4(a), and Fig. S4(b) are the intensity maps of the inelastic neutron scattering data of $Ba_3Yb_2Zn_5O_{11}$ with $E_i$ = 15 meV measured at temperatures 0.25 K and 10 K.

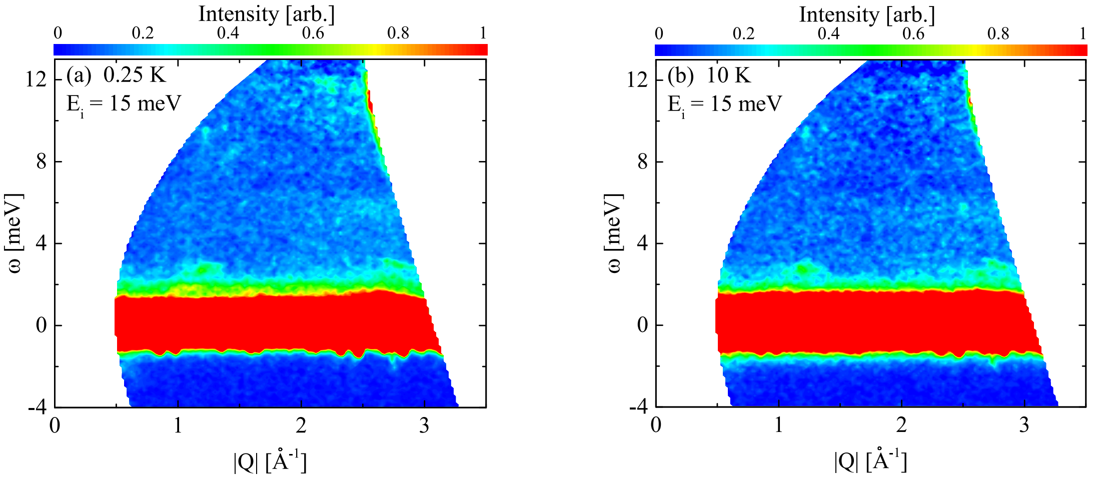


FIG. S4. Intensity map of the inelastic neutron scattering from $Ba_3Yb_2Zn_5O_{11}$ with $E_{\rm i}$ = 15 meV at 0.25 K (a) and 10 K (b).

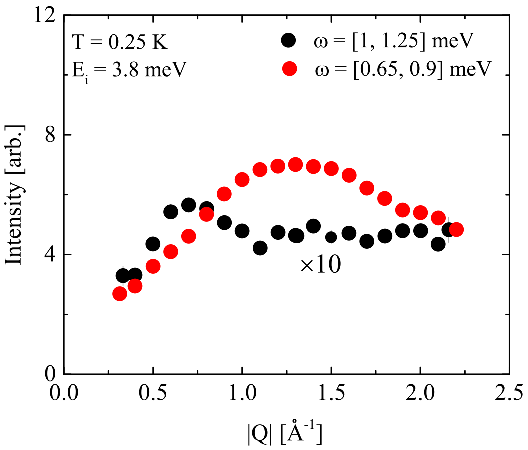


FIG. S5. Wave vector $|\mathbf{Q}|$ dependent neutron scattering intensity measured at 0.25 K with incident energy $E_{\rm i}$ = 3.8 meV, averaged over the excitation energy window $\omega = [0.65, 0.9]$ meV (red points) and $\omega = [1, 1.25]$ meV (black points).

Although the low energy excitations are not well resolved with $E_{\rm i}$ = 15 meV, the data shown in Fig. S4 confirm that there is no additional excitations up to 13.75 meV, which is consistent with the model described in the main text.

As mentioned in the main text, we noticed that there is a weak broad feature in the INS spectrum near an energy transfer of 1 meV (main text Fig. 2(a)). However, this feature has a significantly different dependence on wave vector $|\mathbf{Q}|$ from that of the other observed modes. Fig. S5 shows the wave vector $|\mathbf{Q}|$ dependent neutron scattering intensity measured at 0.25 K with incident energy $E_{\rm i}$ = 3.8 meV, averaged over the excitation energy window $\omega = [0.65, 0.9]$ meV and $\omega = [1, 1.25]$ meV. In contrast to the well defined inelastic mode contained in the energy range $\omega = [0.65, 0.9]$ meV, which peaks near $|\mathbf{Q}| = 1.3\text{Å}^{-1}$, the broad feature captured by the integration range, $\omega = [1, 1.25]$ meV is much weaker with a small peak around $|\mathbf{Q}| = 0.7\text{Å}^{-1}$.

As a supplement to the data collected at 0.25 K and 20 K with $E_{\rm i}$ = 3.8 meV described and shown in the main text, data collected with $E_{\rm i}$ = 3.8 meV at 10 K is shown in Fig. S6 below. The HYSPEC instrumental energy resolution with $E_{\rm i}$ = 3.8 meV and the 180 Hz chopper setting used experimentally is shown in Fig. S7 as a function of energy transfer. The $|\mathbf{Q}|$ dependence of the inelastic spectrum is shown through a series of cuts with an energy range of [0.65, 0.9] meV at temperatures of 0.25, 10, and 20 K in Fig. S8.

## V. CRYSTAL FIELD EXCITATIONS

Inelastic neutron scattering data was collected with the ARCS [S6] time-of-flight spectrometer to probe the excitation spectrum at higher energies. This data was collected at 10 K with $E_{\rm i}$ = 100 meV and shows three crystal field excitations at ∼ 38, 54, and 67 meV. The data presented here are consistent with the results of Ref. [S7] where a more detailed analysis of the crystal field excitation spectrum and Hamiltonian can be found. We note that for a Kramers ion such as $Yb^{3+}$ ($J = 7/2$), in the absence of broken time reversal symmetry, the minimum degeneracy is two so that $(2J+1)/2$ doublets are expected including the ground state. Thus the observation of three crystal field excitations is strong evidence that the modes observed at energies less than ∼ 2 meV discussed in the main paper are due to interactions between the $Yb^{3+}$ within each tetrahedron.

## VI. THEORETICAL DETAILS

### A. Model

For completeness, we state our model and conventions in more detail. We consider the effective anistoropic exchange

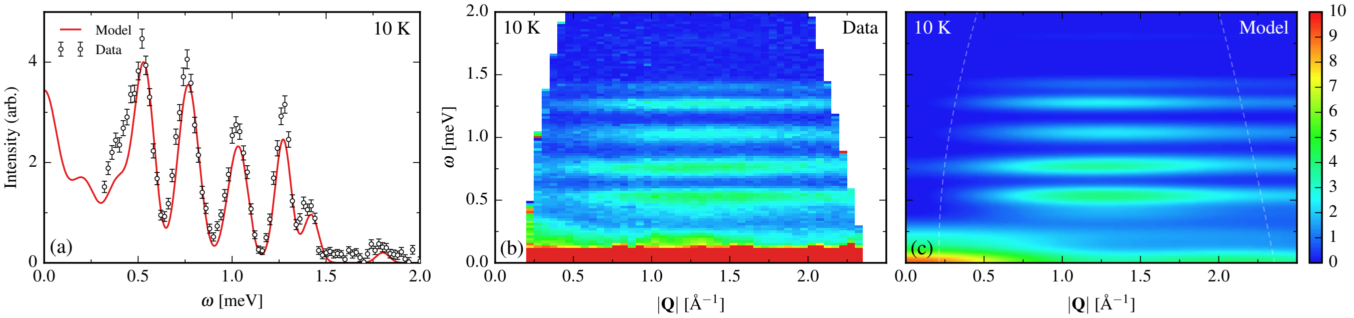


FIG. S6. Inelastic neutron scattering data ($E_i$=3.8 meV) and comparison to theoretical model at (a-c) 10 K. The overall theoretical intensity scale was fit using the INS cut at 0.25 K. A Gaussian broadening with energy dependence following the experimental energy resolution function (shown in Fig. S7) was included in the theoretical calculation. (a) Cut of INS data averaged over the window $1.25\text{Å}^{-1} < |\mathbf{Q}| < 1.35\text{Å}^{-1}$. Results for the best fit single tetrahedron model of the main text are shown. (b) Intensity map of powder averaged INS data. The excitations are nearly dispersion free over the full $|\mathbf{Q}|$ range. (c) Model calculations for the best fit single tetrahedron model. The $Yb^{3+}$ form factor was evaluated in the dipole approximation, as given in Ref. [S4].

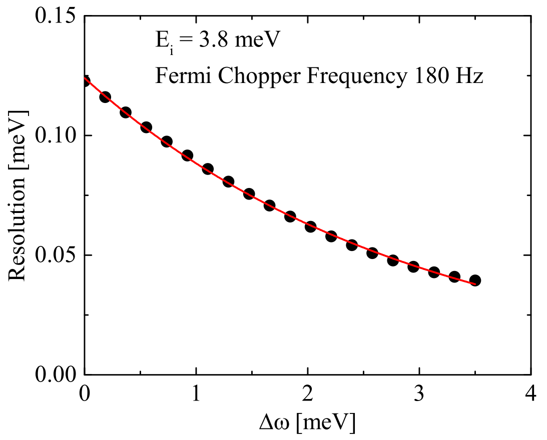


FIG. S7. HYSPEC resolution as a function of the energy transfer $\Delta\omega$, with incident energy $E_\mathrm{i} = 3.8$ meV and Fermi chopper frequency of 180 Hz. The red line is the fit to the empirical equation $y = Ae^{-\Delta\omega/\Gamma}$ with $A = 0.12398 \pm 0.0004$ meV, and $\Gamma = 2.95111 \pm 0.02144$ meV.

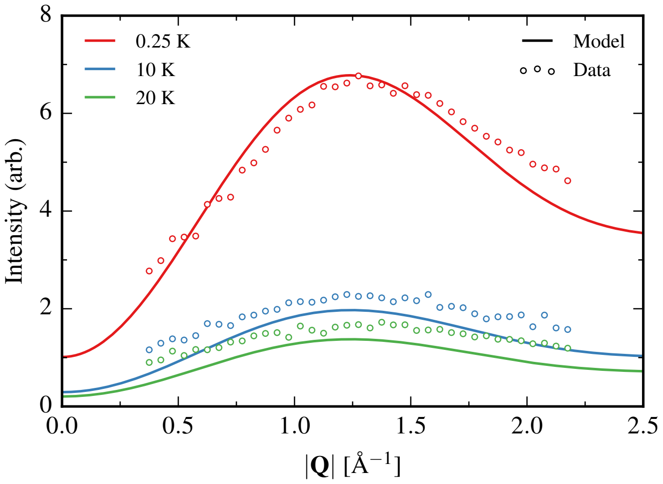


FIG. S8. The $|\mathbf{Q}|$ dependence of the inelastic neutron scattering data for $Ba_3Yb_2Zn_5O_{11}$, averaged over the excitation in the energy window $0.65\text{ meV} < \omega < 0.9$ meV.

model in the local basis defined as

$$\begin{aligned} H_{\text{eff}} \equiv \sum_{i=1}^{4}\sum_{j<i}\Big[J_{zz}S_i^zS_j^z - J_{\pm}\left(S_i^+S_j^- + S_i^-S_j^+\right) + \\ J_{\pm\pm}\left(\gamma_{ij}S_i^+S_j^+ + \text{h.c}\right) + J_{z\pm}\left(\zeta_{ij}\left[S_i^zS_j^+ + S_i^+S_j^z\right] + \text{h.c}\right)\Big] \\ -\mu_B\mathbf{B}\cdot\sum_{i=1}^{4}\left[g_{\pm}\left(\hat{\mathbf{x}}_iS_i^x + \hat{\mathbf{y}}_iS_i^y\right) + g_z\hat{\mathbf{z}}_iS_i^z\right], \end{aligned} \tag{S1}$$

with four symmetry allowed exchanges $J_{zz}$, $J_{\pm}$, $J_{\pm\pm}$ and $J_{z\pm}$ and external magnetic field $\mathbf{B}$. The complex bond phase factors $\gamma_{ij}$ and $\zeta_{ij} = -\gamma_{ij}^*$ depend only on the basis sites they connect and thus can be expressed as a matrix

$$\gamma = \begin{pmatrix} 0 & +1 & \omega & \omega^2 \\ +1 & 0 & \omega^2 & \omega \\ \omega & \omega^2 & 0 & +1 \\ \omega^2 & \omega & +1 & 0 \end{pmatrix}, \tag{S2}$$

where $\omega = e^{2\pi i/3}$. The magnetic field is coupled directly to the effective moment on each $Yb^{3+}$ site, defined as

$$\boldsymbol{\mu}_i \equiv \mu_B\left[g_{\pm}\left(\hat{\mathbf{x}}_iS_i^x + \hat{\mathbf{y}}_iS_i^y\right) + g_z\hat{\mathbf{z}}_iS_i^z\right], \tag{S3}$$

where $g_z$ and $g_{\pm}$ are the $g$-factors in the local [111] direction and in the plane perpendicular to it. These local axes are de-

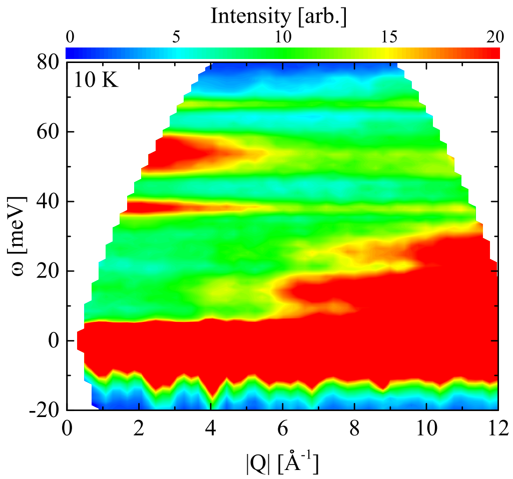


FIG. S9. Intensity map of the inelastic neutron scattering data from $Ba_3Yb_2Zn_5O_{11}$ with $E_\mathrm{i}$ = 100 meV at 10 K . The data shows three crystal field excitations at 38, 54, and 67 meV.

fined as

$$
\begin{aligned}
\hat{\mathbf{z}}_1 &= \frac{1}{\sqrt{3}}(+\hat{\mathbf{x}}+\hat{\mathbf{y}}+\hat{\mathbf{z}}), \quad & \hat{\mathbf{x}}_1 &= \frac{1}{\sqrt{6}}(-2\hat{\mathbf{x}}+\hat{\mathbf{y}}+\hat{\mathbf{z}}),\\
\hat{\mathbf{z}}_2 &= \frac{1}{\sqrt{3}}(+\hat{\mathbf{x}}-\hat{\mathbf{y}}-\hat{\mathbf{z}}), \quad & \hat{\mathbf{x}}_2 &= \frac{1}{\sqrt{6}}(-2\hat{\mathbf{x}}-\hat{\mathbf{y}}-\hat{\mathbf{z}}),\\
\hat{\mathbf{z}}_3 &= \frac{1}{\sqrt{3}}(-\hat{\mathbf{x}}+\hat{\mathbf{y}}-\hat{\mathbf{z}}), \quad & \hat{\mathbf{x}}_3 &= \frac{1}{\sqrt{6}}(+2\hat{\mathbf{x}}+\hat{\mathbf{y}}-\hat{\mathbf{z}}),\\
\hat{\mathbf{z}}_4 &= \frac{1}{\sqrt{3}}(-\hat{\mathbf{x}}-\hat{\mathbf{y}}+\hat{\mathbf{z}}), \quad & \hat{\mathbf{x}}_4 &= \frac{1}{\sqrt{6}}(+2\hat{\mathbf{x}}-\hat{\mathbf{y}}+\hat{\mathbf{z}}),
\end{aligned} \tag{S4}
$$

where $\hat{\mathbf{y}}_i = \hat{\mathbf{z}}_i \times \hat{\mathbf{x}}_i$.

Equivalently, this model can be expressed in *global* quantization axes [S8]. We thus define a global pseudo-spin operator $\tilde{\mathbf{S}}_i$ for each $Yb^{3+}$ site as

$$
\tilde{\mathbf{S}}_i \equiv \hat{\mathbf{x}}_i S_i^x + \hat{\mathbf{y}}_i S_i^y + \hat{\mathbf{z}}_i S_i^z. \tag{S5}
$$

In this basis the anisotropic exchange model can be written

$$
H_\mathrm{eff} \equiv \sum_{j=1}^{4} \sum_{i<j} \tilde{\mathbf{S}}_i^\intercal \mathbf{J}_{ij} \tilde{\mathbf{S}}_j, \tag{S6}
$$

where the exchange matrices $\mathbf{J}_{ij}$ are defined as

$$
\begin{aligned}
\mathbf{J}_{12} &= \begin{pmatrix} J_2 & J_4 & J_4 \\ -J_4 & J_1 & J_3 \\ -J_4 & J_3 & J_1 \end{pmatrix}, \quad & \mathbf{J}_{13} &= \begin{pmatrix} J_1 & -J_4 & J_3 \\ J_4 & J_2 & J_4 \\ J_3 & -J_4 & J_1 \end{pmatrix},\\
\mathbf{J}_{14} &= \begin{pmatrix} J_1 & J_3 & -J_4 \\ J_3 & J_1 & -J_4 \\ J_4 & J_4 & J_2 \end{pmatrix}, \quad & \mathbf{J}_{23} &= \begin{pmatrix} J_1 & -J_3 & J_4 \\ -J_3 & J_1 & -J_4 \\ -J_4 & J_4 & J_2 \end{pmatrix},\\
\mathbf{J}_{24} &= \begin{pmatrix} J_1 & J_4 & -J_3 \\ -J_4 & J_2 & J_4 \\ -J_3 & -J_4 & J_1 \end{pmatrix}, \quad & \mathbf{J}_{34} &= \begin{pmatrix} J_2 & -J_4 & J_4 \\ J_4 & J_1 & -J_3 \\ -J_4 & -J_3 & J_1 \end{pmatrix}.
\end{aligned} \tag{S7}
$$

These two different parametrizations are related as

$$
\begin{aligned}
J_1 &= \frac{1}{3}\left(+4J_\pm + 2J_{\pm\pm} + 2\sqrt{2}J_{z\pm} - J_{zz}\right),\\
J_2 &= \frac{1}{3}\left(-4J_\pm + 4J_{\pm\pm} + 4\sqrt{2}J_{z\pm} + J_{zz}\right),\\
J_3 &= \frac{1}{3}\left(-2J_\pm - 4J_{\pm\pm} + 2\sqrt{2}J_{z\pm} - J_{zz}\right),\\
J_4 &= \frac{1}{3}\left(-2J_\pm + 2J_{\pm\pm} - \sqrt{2}J_{z\pm} - J_{zz}\right).
\end{aligned} \tag{S8}
$$

As discussed in the main text, the exchange $J_4$ can be interpreted as a Dzyaloshinskii-Moriya (DM) interaction. Specifically, for $J_1 = J_2 \equiv J$ and $J_3 = 0$ we can write

$$
H_\mathrm{eff} = \sum_{j=1}^{4} \sum_{i<j} \left[ J\tilde{\mathbf{S}}_i \cdot \tilde{\mathbf{S}}_j + \mathbf{D}_{ij} \cdot \left(\tilde{\mathbf{S}}_i \times \tilde{\mathbf{S}}_j\right)\right], \tag{S9}
$$

where the DM vectors are defined as $\mathbf{D}_{ij} \equiv D\hat{\mathbf{D}}_{ij}$ with magnitude $D = \sqrt{2}J_4$ and directions

$$
\begin{aligned}
\hat{\mathbf{D}}_{12} &= \frac{-\hat{\mathbf{y}}+\hat{\mathbf{z}}}{\sqrt{2}}, \quad & \hat{\mathbf{D}}_{13} &= \frac{+\hat{\mathbf{x}}-\hat{\mathbf{z}}}{\sqrt{2}}, \quad & \hat{\mathbf{D}}_{14} &= \frac{-\hat{\mathbf{x}}+\hat{\mathbf{y}}}{\sqrt{2}},\\
\hat{\mathbf{D}}_{23} &= \frac{-\hat{\mathbf{x}}-\hat{\mathbf{y}}}{\sqrt{2}}, \quad & \hat{\mathbf{D}}_{24} &= \frac{+\hat{\mathbf{x}}+\hat{\mathbf{z}}}{\sqrt{2}}, \quad & \hat{\mathbf{D}}_{34} &= \frac{-\hat{\mathbf{y}}-\hat{\mathbf{z}}}{\sqrt{2}}.
\end{aligned} \tag{S10}
$$

With these definitions $J_4 > 0$ corresponds to the so-called direct case, while $J_4 < 0$ corresponds to the indirect case [S9].

### B. Observables

The effective single tetrahedron model can be numerically diagonalized exactly and all observable quantities can be directly computed. Below we outline how each observable is computed and compared with the respective experimental results.

#### 1. *Specific heat*

As the lattice contribution has been subtracted in Ref. [S1] using the structural analog $Ba_3Lu_2Zn_5O_{11}$, we simply compute the magnetic contribution directly from the model. This is straightforwardly

$$
C = \frac{1}{4}\left(\frac{\langle H_\mathrm{eff}^2\rangle - \langle H_\mathrm{eff}\rangle^2}{k_B T^2}\right), \tag{S11}
$$

where $\langle O\rangle = \mathrm{tr}[Oe^{-\beta H_\mathrm{eff}}]/\mathrm{tr}[e^{-\beta H_\mathrm{eff}}]$ denotes a thermal average. While the lattice subtraction seems robust, we only use the specific heat data of Kimura *et al.* [S1] below $T < 5$ K to minimize any possible bias from this procedure.

#### 2. *Susceptibility*

We compute the magnetic susceptibility by emulating the experimental procedure of Kimura *et al.* [S1]. We thus add

a small magnetic field with $|\mathbf{B}| = 0.1$ T and the compute magnetization, $\boldsymbol{\mu} \equiv 1/4 \sum_{i=1}^{4} \boldsymbol{\mu}_i$, in the effective single tetrahedron model. To better compare to the experimental results, we need to include Van Vleck contributions from the higher crystal field levels and the diamagnetic susceptibility from the $Yb^{3+}$ core electrons. At these low temperatures, we treat this as a constant shift $\chi_0$ to be added to $\chi$. Estimates from Ref. [S1] place these contributions at roughly $\chi_0 \sim 6.9 \cdot 10^{-3}$ emu/(mol Yb), though we leave $\chi_0$ as a free parameter in our analysis. As we will see below, the fitted value of $\chi_0$ agrees well with this theoretical estimate. In total the susceptibility, $\chi$, is given by

$$\chi \equiv \mu_0 |\langle \boldsymbol{\mu} \rangle| / |\mathbf{B}| + \chi_0, \tag{S12}$$

where $\langle \boldsymbol{\mu} \rangle$ is the magnetization computed in the effective single tetrahedron model in the presence of the magnetic field $\mathbf{B}$. Due to the cubic symmetry, the susceptibility is isotropic and thus the direction $\hat{\mathbf{B}}$ of this applied field is unimportant. We have verified that this field is well within the linear regime, with essentially no difference in computing $\chi$ with an extremely small field of $|\mathbf{B}| = 10^{-3}$ T rather than $|\mathbf{B}| = 0.1$ T.

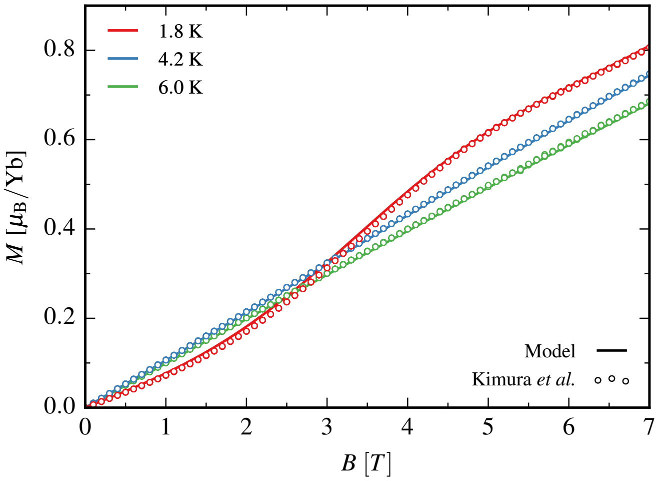


FIG. S10. Comparison of the magnetization data of Kimura *et al.* [S1] at $T = 1.8$ K, 4.2 K and 6.0 K to the model calculations for the best fit parameters. The Van Vleck and core diamagnetic contributions, $\chi_0$, fitted in the susceptibility also contribute to the magnetization.

### 3. *Magnetization*

To compare to the magnetization data of Kimura *et al.* [S1] at larger fields, we compute the magnetization itself as a function of field. As in computing the susceptibility, the $\chi_0$ shift contributes a linear correction to magnetization computed directly from the single tetrahedron model. Explicitly, the total magnetization $\mathbf{M}$ per $Yb^{3+}$ is given as

$$\mathbf{M} \equiv \langle \boldsymbol{\mu} \rangle + \chi_0 \mathbf{B}/\mu_0, \tag{S13}$$

where $\langle \boldsymbol{\mu} \rangle$ is the magnetization computed in the effective single tetrahedron model. Unlike when computing the susceptibility, the magnetization measurements of Ref. [S1] go beyond the linear regime and thus $\langle \boldsymbol{\mu} \rangle$ *does* depend on the field direction $\hat{\mathbf{B}}$. To emulate the inherent averaging in the powder samples, we consider fields with arbitrary direction $\hat{\mathbf{B}}$ and fixed magnitude $|\mathbf{B}|$. For each $\mathbf{B}$ we then compute $\hat{\mathbf{B}} \cdot \mathbf{M}$ and integrate over field directions $\hat{\mathbf{B}}$ to obtain the contribution to the powder averaged magnetization.

### 4. *Inelastic neutron scattering*

The inelastic neutron scattering intensity is given by

$$I(\mathbf{Q}, \omega) = I_0 \frac{|\mathbf{k}'|}{|\mathbf{k}|} \sum_{\alpha\beta} \left( \delta_{\alpha\beta} - \hat{Q}_\alpha \hat{Q}_\beta \right) F(|\mathbf{Q}|)^2 \mathcal{S}^{\alpha\beta}(\mathbf{Q}, \omega), \tag{S14}$$

where $\mathbf{k}$, $\mathbf{k}'$ are the initial and final neutron momenta, $F(Q)$ is the form factor for $Yb^{3+}$ [S4] and $I_0$ is a normalization factor. The dynamical structure factor for a single tetrahedron, $\mathcal{S}^{\alpha\beta}(\mathbf{Q}, \omega)$, is given as

$$\mathcal{S}^{\alpha\beta}(\mathbf{Q}, \omega) = \sum_{nn'} \frac{e^{-\beta E_n}}{Z} \langle n | \mu^\alpha_{-\mathbf{Q}} | n' \rangle \langle n' | \mu^\beta_{\mathbf{Q}} | n \rangle \, \delta(\omega - E_{n'} + E_n),$$

where $|n\rangle$, $E_n$ are the eigenstates and energies of the single tetrahedron model $H_{\text{eff}}$ and $Z$ is the partition function. The operators $\boldsymbol{\mu}_{\mathbf{Q}}$ are defined as

$$\boldsymbol{\mu}_{\mathbf{Q}} \equiv \frac{1}{4} \sum_{i=1}^{4} e^{-i\mathbf{Q}\cdot\mathbf{r}_i} \boldsymbol{\mu}_i, \tag{S15}$$

where $\boldsymbol{\mu}_i$ and $\mathbf{r}_i$ are the $Yb^{3+}$ moments and site positions. The prefactor $|\mathbf{k}'|/|\mathbf{k}| = (1 - \omega/E_{\text{i}})^{1/2}$ and reduces the relative intensity of some higher lying features. For the INS data we are interested in, one has $E_{\text{i}} = 3.8$ meV and this only is significant at high energies. We consider the powder averaged cross section

$$I_{\text{avg}}(Q, \omega) \equiv \int d\hat{\mathbf{Q}} \; I(Q\hat{\mathbf{Q}}, \omega). \tag{S16}$$

Due to the isolated tetrahedra, strictly $I_{\text{avg}}(Q, \omega)$ has features flat in $|\mathbf{Q}|$, and sharp in energy. At low temperature, these simply reflect transitions from the ground state to the excited levels. Additional information resides in the intensity variations. To compare with the experimental data, we include an overall scale factor, $I_0$, to represent the arbitrary experimental intensity scale. To emulate the finite experimental energy resolution, we convolve $I_{\text{avg}}(Q, \omega)$ with Gaussians of finite width. The experimental energy resolution is energy dependent, varying approximately as $\sim Ae^{-\omega/\Gamma}$ as given in Fig. S7. To incorporate this, the width of this Gaussian broadening made energy dependent as well, following this experimental form. However, as the observed levels are somewhat broader than the experimental limit, we allow the overall scale of this energy dependent width, denoted as $A^{(\text{fit})}$, to vary in the theoretical calculation while keeping the experimentally determined value for $\Gamma$.

### C. Fitting

As discussed in the main text, to fit the experimental data we use the specific heat, susceptibility and a cut of inelastic neutron scattering data averaged over the range $1.25\text{Å}^{-1} < |\mathbf{Q}| < 1.35\text{Å}^{-1}$. Here we present explicit details of our fitting methodology. We denote the specific heat data of Kimura *et al.* [S1] as a set of temperatures $T_n^{(\mathrm{exp},C)}$ and values $C_n^{(\mathrm{exp})}$ where $n$ labels each data point. As discussed in the main text, we only use data points with $T < 5$ K to minimize possible issues with the lattice subtraction. Similarly for the susceptibility, we define $T_n^{(\mathrm{exp},\chi)}$ and $\chi_n^{(\mathrm{exp})}$ (taking all points with $T < 30$ K) and for the INS cut $\omega_n^{(\mathrm{exp},\chi)}$ and $I_n^{(\mathrm{exp})}$ (taking all points with 0.25 meV $< \omega <$ 2 meV in the $T = 0.25$ K cut). For each temperature $T$ or energy $\omega$ we can compute the theoretical values, yielding $C_n^{(\mathrm{theo})}$, $\chi_n^{(\mathrm{theo})}$ and $I_n^{(\mathrm{theo})}$ as outlined in the previous section. Thinking of these sets of observations and theoretical values as vectors, we define the discrepancy

$$\epsilon_X \equiv |\mathbf{X}^{(\mathrm{exp})} - \mathbf{X}^{(\mathrm{theo})}|/|\mathbf{X}^{(\mathrm{exp})}|, \quad \text{(S17)}$$

where $X = C, \chi$ or $I$. To find the best fit of the experimental data, we minimize the sum of these differences $\epsilon_{\mathrm{tot}} \equiv \epsilon_C + \epsilon_\chi + \epsilon_I$. In total we have nine fitting parameters:

1. The exchanges $J_{zz}$, $J_\pm$, $J_{\pm\pm}$ and $J_{z\pm}$
2. The $g$-factors, $g_z$ and $g_\pm$
3. The susceptibility shift $\chi_0$
4. The intensity scale of the INS spectrum $I_0$ and the scale of the Gaussian energy broadening $A^{(\mathrm{fit})}$

We used standard minimization algorithms to find the best fit presented in the main text. To aid in finding the global minimum, the minimization process was repeated for several thousand random initial conditions. To be specific regarding the initialization, the four exchanges were drawn from uniform distributions covering the range $[-0.3, +0.3]$ meV, each $g$-factor from the range $[1, 3]$ and $\chi_0$ susceptibility shift from the range $[6, 8] \cdot 10^{-3}$ emu/(mol Yb). The neutron intensity was always initialized to $I_0 = 0.01$, while the energy width $A^{(\mathrm{fit})}$ was initialized with the experimental value $A = 0.124$ meV. In the main text, we reported the exchanges and $g$-factors. The remaining parameters for the best fit are given as

$$I_0 = 0.012, \quad A^{(\mathrm{fit})}/A = 1.24, \quad \chi_0 = 6.75 \cdot 10^{-3}\ \text{emu/(mol Yb)}.$$

We see that the susceptibility shift $\chi_0$ compares favorably with the expected theoretical value [S1]. We note that the required scale to the energy broadening is somewhat larger than the experimental resolution, by about 25%, as can be seen directly in the INS cuts at 0.25 K. Additional comparisons of the experimental results and the theoretical model are shown in Fig. S6 (INS at 10 K), Fig. S10 (magnetization) and Fig. S8 ($|\mathbf{Q}|$ dependence of INS intensity).

While the best fit parameters found are qualitatively unique, they can vary somewhat if one changes details of the fitting procedure. For example, by changing temperature ranges used in $C$ or $\chi$, or assigning different relative weights to each data set. The most sensitive of the parameters is $J_{zz}$, which can vary by as much as 0.02 to 0.04 meV, while the other parameters can vary by 10% or so. None of these variations change the qualitative picture that emerges from our analysis; in the global basis the system predominantly antiferromagnetic Heisenberg and (indirect) DM interactions and small symmetric anisotropies.


[S1] K. Kimura, S. Nakatsuji, and T. Kimura, Phys. Rev. B **90**, 060414 (2014).

[S2] A. Huq, J. P. Hodges, L. Heroux, and O. Gourdon, Zeitschrift fur Kristallographie Proceedings **1**, 127 (2011).

[S3] J. Rodriguez-Carvajal, Physica B: Condensed Matter **192**, 55 (1993).

[S4] A. J. C. Wilson, *International Tables for Crystallography: Mathematical, physical, and chemical tables*, Vol. 3 (International Union of Crystallography, 1992).

[S5] B. Winn, U. Filges, V. O. Garlea, M. Graves-Brook, M. Hagen, C. Jiang, M. Kenzelmann, L. Passell, S. M. Shapiro, X. Tong, and I. Zaliznyak, in *EPJ Web of Conferences*, Vol. 83 (EDP Sciences, 2015) p. 03017.

[S6] D. L. Abernathy, M. B. Stone, M. J. Loguillo, M. S. Lucas, O. Delaire, X. Tang, J. Y. Y. Lin, and B. Fultz, Review of Scientific Instruments **83**, 015114 (2012).

[S7] T. Haku, M. Soda, M. Sera, K. Kimura, S. Itoh, T. Yokoo, and T. Masuda, (2015), arXiv:1510.03049 [cond-mat.mtrl-sci].

[S8] H. Yan, O. Benton, L. D. C. Jaubert, and N. Shannon, (2013), arXiv:1311.3501 [cond-mat.str-el].

[S9] B. Canals, M. Elhajal, and C. Lacroix, Phys. Rev. B **78**, 214431 (2008).
